# Supplementary material for: MLCommons Chakra: Advancing Performance Benchmarking and Co-design using Standardized Execution Traces
Source: arXiv:2605.11333 source file (2026-05-19)
Supplement: Supplementary file 1 [file additional_results.tex]

% \FloatBarrier
\newpage
\section{Appendix: Additional Results}
\label{sec:additional_results}

\subsection{Inference System Scalability Analysis using ASTRA-sim}

In this experiment, we simulate the deepseek-R1 inference system~\cite{deepseekV3R1_inference_system_2025} under different parallelism strategy for the scalability of prefill and decode independently. We assume a system composed of 64x8 H100 DGX GPUs, and a global batch size of 2048. The system is partitioned into smaller clusters, ranging from four clusters with 128 GPUs, to 16 clusters with 32 GPUs each, with the batch size divided proportionally across clusters.We vary two parallelism axes in our experiments: 1) EP/DP, where we do expert-parallel for routed experts and data-parallel for remain layers, 2) TP, where we apply tensor-parallel for all layers. We separate prefilling and decoding stages as they may prefer a different system, where prefilling has a sequence length of 1K, and decoding has a KV cache of 64K tokens.

~\autoref{tab:astra_scaling_expr_table} shows the end-to-end runtime of each system and parallel strategies. The EP/DP can be calculated by dividing cluster size and TP. From the results we can observe two points: 1) For either prefilling or decoding, appropriately increase tensor-parallel can reduce runtime, as it equivalently increase batch size and improve operational intensity. However, excessive tensor-parallelism introduces significant communication overhead compared to EP/DP, which can offset or even hide the potential speedup. 2) For prefilling stage, the system scale do not affect the runtime much, while decoding is more sensitive to system scale. Under the long-context decoding, a larger system results in a longer runtime. 

\begin{table}[!t]
  \caption{Deepseek-R1 inference simulation, different cluster size and parallel strategies}
  \centering
  \resizebox{\columnwidth}{!}{%
  \begin{tabular}{|c|c|c|c|c|c|c|}
    \hline
    \multirow{2}{*}{\diagbox{TP}{GPUs}}    & \multicolumn{3}{c|}{Prefilling} & \multicolumn{3}{c|}{Decoding}     \\
    \cline{2-7}
           & 16x32     & 8x64      & 4x128     & 16x32     & 8x64      & 4x128     \\
    \hline
     1     & 357.495   &  360.255  & 377.059   & 1006.680  &  1120.404 & 1195.683  \\
     \hline
     2     & 373.289   &  431.517  & 646.562   & 643.583   & 756.911   & 813.572   \\
     \hline
     4     & 180.834   &  195.016  & 248.261   & 362.799   & 401.736   & 508.196   \\
     \hline
     8     & 204.070   &  208.143  & 222.446   & 379.989   & 400.282   & 463.374   \\
    \hline
     
  \end{tabular}
  }
  \label{tab:astra_scaling_expr_table}
\end{table}

\subsection{Detailed Simulation studies on Scala Computing Platform}

The Scala Compute Platform (SCP) is a high-performance commercial discrete-event simulator developed by Scala Computing and built on ns-3. SCP is used by data center operators and networking equipment manufacturers to perform large-scale Chakra simulations. It runs on on-demand compute clusters in the AWS cloud and supports simulations involving over 100,000 GPUs communicating via RoCEv2 or an enhanced Ethernet Transport (eET) inspired by the Ultra Ethernet Transport (UET) specs~\cite{ultra-ethernet}.

\noindent\textbf{Simulation Sytem.}The simulation is conducted on a system consisting of 256 GPUs. The network topology employs fully provisioned 51.2-Tb/s Ethernet switches organized in a two-tier Clos configuration, featuring 800-Gb/s inter-switch links and 400-Gb/s NICs. The workload is generated using Chakra traces synthesized with a STAGE~\cite{stage}, configured with model dimensions of $d_{\mathrm{in}} = d_{\mathrm{out}} = d_{\mathrm{model}} = 5120$, feed-forward dimension $d_{\mathrm{ffn}} = 13824$, sequence length $8192$, $40$ attention heads, and $80$ stacked transformer layers.
To estimate the computation times for this generated Chakra graphs, it is augmented with NVIDIA A100 profiling data. Workload parallelization is configured as 64 DP × 2 TP × 2 PP × 1 SP. The RDMA transport protocols evaluated include RoCEv2 and eET. Each simulation runs for a duration of 2 seconds and is executed on Scala’s MPI-enhanced ns-3 environment deployed on AWS.

% \insertFigure{what_if_network_bw_dgx}{Communication Time for Different Network Topology and Bandwidth - Mixtral 8x7B}{0.98}{-1em}{-1em}

\subsubsection{Overview}

We simulated an LLM workload on a small, two-tier RDMA network with 256 NVIDIA A100 GPUs. The study evaluated the workload’s performance over RoCEv2 and eET. For RoCEv2, the network was made “lossless” by enabling PFCs. For eET, PFCs were disabled and congestion was managed using NSCC and flow control, both inspired by UET. In addition, eET employed packet spraying with a 128-way spray size. 

A critical feature of LLM workloads is their high degree of synchrony: performance is strongly influenced by within-GPU dependencies between computation and communication operations, as well as cross-GPU dependencies (e.g., \texttt{SEND}/\texttt{RECEIVE}). Chakra’s ability to capture these dependencies is essential for accurate simulation of LLM workloads.

\subsubsection{Analysis and Metrics}
The metrics in this study include: (i) the distribution of NIC transmit–link utilization, (ii) aggregated NIC receive throughput, (iii) RTTs, (iv) congestion statistics and plots for PFC and NSCC, and (v) workload progress toward completion measured by the CDF of send bytes. For detailed analysis of (iii), (iv) and (v), it is included in the appendix attached with this submission.

\subsubsection{NIC Transmit/Receive Link Utilization}
The distribution of NICs by transmit utilization is shown in the \emph{Tx link utilization} heatmap \autoref{fig:SCALA_UET_NIC_RX_TX}(a) and \autoref{fig:SCALA_RoCE_NIC_RX_TX}(a). 
The y-axis reports utilization percentage, and the x-axis shows simulation time. Color encodes the count of NICs at each utilization level, with dark red indicating the maximum (256) and dark blue indicating zero. Notably, after 300\,ms for RoCEv2 and 500\,ms for eET, a large fraction of NICs are no longer transmitting at high rates. This arises from the synchronous nature of LLM workloads: prolonged intervals of low network utilization reflect GPUs spending substantial time on computation rather than communication (due to the nature of more DP than TP and PP in the experiment setup) or waiting to receive data from other GPUs.

Considering the receive-side NICs, we observe oscillatory behavior driven by the workload structure \autoref{fig:SCALA_UET_NIC_RX_TX}(b) and \autoref{fig:SCALA_RoCE_NIC_RX_TX}(b). Even with a fully provisioned topology, the average link utilization remains well below the 400\,Gb/s line rate, with extended periods of underutilization while GPUs are computing or waiting on dependencies.

\insertFigure{SCALA_UET_NIC_RX_TX}{Results of eET v2 NIC Transmit Receive}{0.98}{-1em}{-1em}

%\insertFigure{SCALA_RoCE_NIC_RX_TX}{Results of RoCE v2 NIC Transmit Receive}{0.98}{-1em}{-2em}
% \begin{figure*}[htbp]
%     \centering
%     \begin{subfigure}[b]{0.45\textwidth}
%         \centering
%         \includegraphics[width=\textwidth]{figures/Scala_ROCE_NIC_Tx_Link_Utilization.png}
%         \caption{ROCEv2}
%     \end{subfigure}
%     \hfill
%     \begin{subfigure}[b]{0.45\textwidth}
%         \centering
%         \includegraphics[width=\textwidth]{figures/Scala_UET_NIC_Tx_Link_Utilization.png}
%         \caption{UET}
%     \end{subfigure}
%     \caption{Transmit Link Utilization}
% \end{figure*}

% \begin{figure*}[h!]
%     \centering
%     \begin{subfigure}[b]{0.45\textwidth}
%         \centering
%         \includegraphics[width=\textwidth]{figures/Scala_ROCE_NIC_Aggregated_NIC_Rx_Throughput.png}
%         \caption{ROCEv2}
%     \end{subfigure}
%     \hfill
%     \begin{subfigure}[b]{0.45\textwidth}
%         \centering
%         \includegraphics[width=\textwidth]{figures/Scala_UET_Aggregated_NIC_Rx_Throughput.png}
%         \caption{UET}
%     \end{subfigure}
%     \caption{Aggregated NIC Rx Throughput}
% \end{figure*}

\subsubsection{Round Trip Times}
RTT traces for both RoCEv2 and eET show periodic peaks, indicating congestion in the network. Although mean RTTs are low, RoCEv2 exhibits significantly higher peaks, above 1\,ms, whereas eET peaks are around 25\,\textmu s \autoref{fig:RTT}. This is consistent with UET NSCC aggressively keeping switch buffers shallow, whereas RoCEv2 relies on PFCs. Higher tail latencies can degrade the performance of tightly synchronized workloads such as LLMs.

\begin{figure*}[htbp]
    \centering
    \begin{subfigure}[b]{0.45\textwidth}
        \centering
        \includegraphics[width=\textwidth]{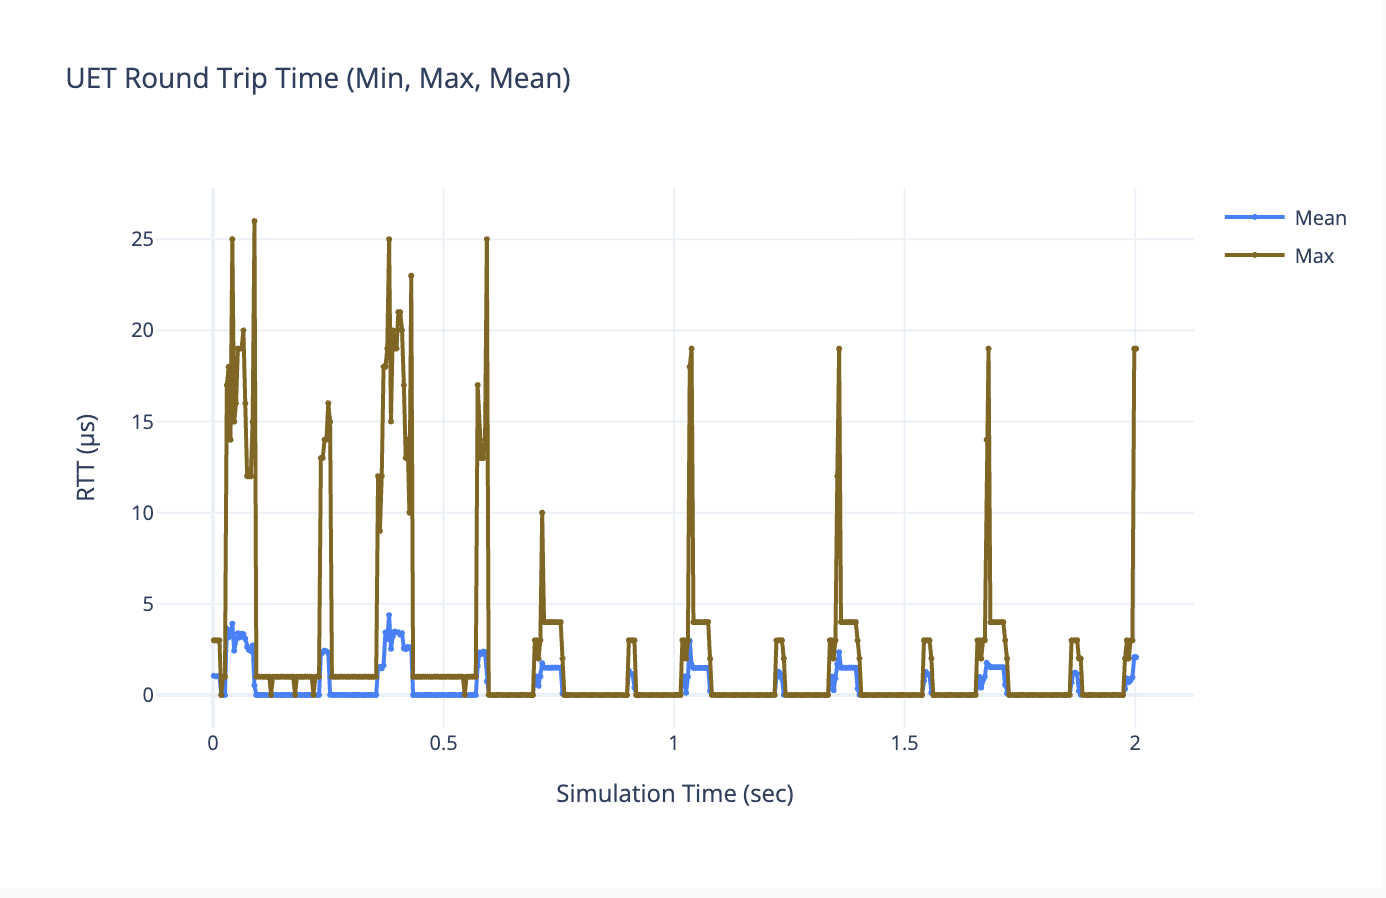}
        \caption{eET RTT}
    \end{subfigure}
    \hfill
    \begin{subfigure}[b]{0.45\textwidth}
        \centering
        \includegraphics[width=\textwidth]{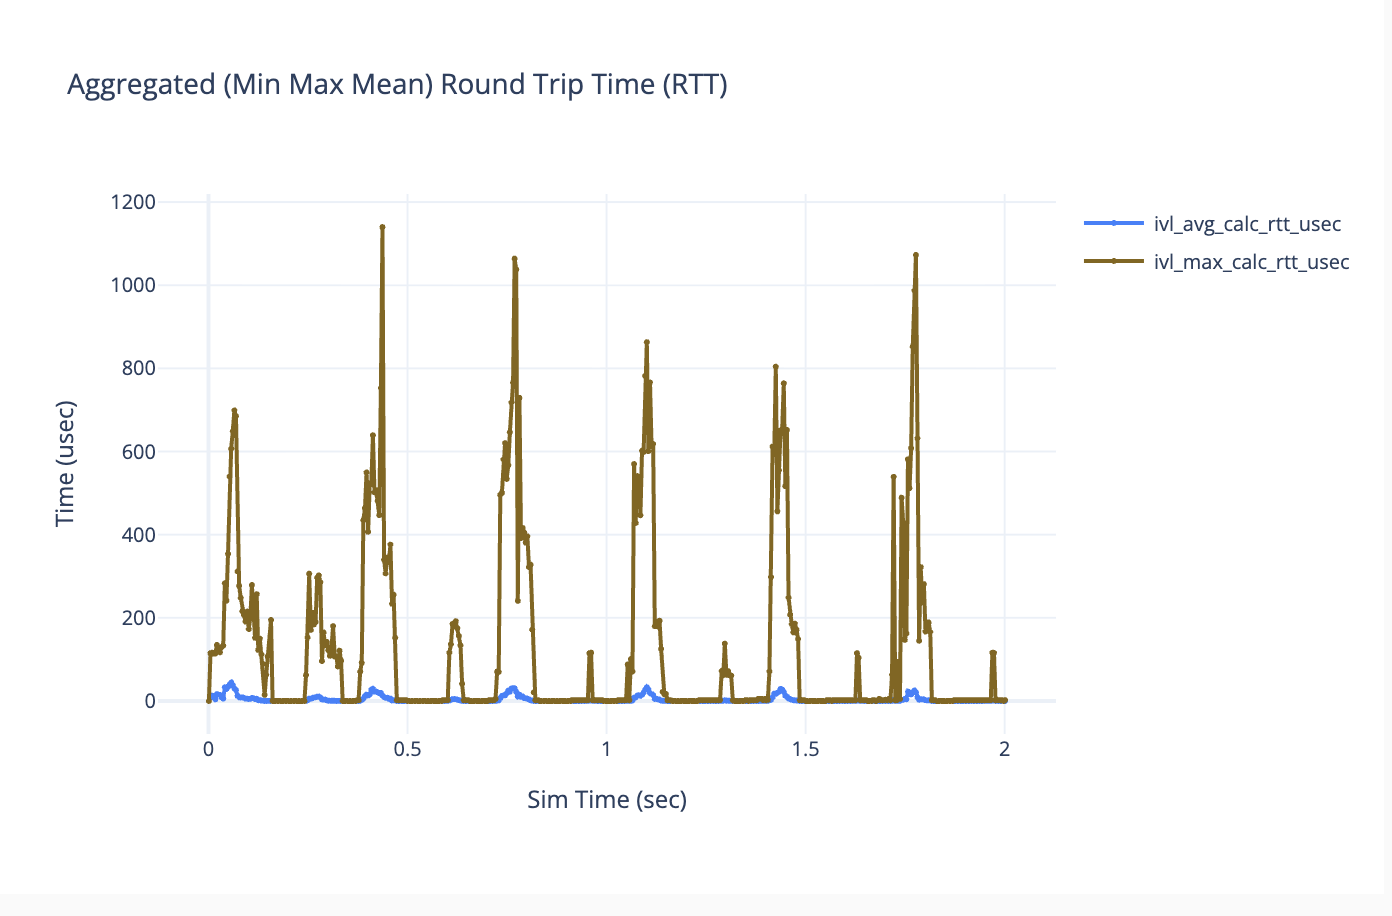}
        \caption{RoCE RTT}
    \end{subfigure}
    \caption{eET and RoCE RTT (with Mean and Max)}
    \label{fig:RTT}
\end{figure*}

\subsubsection{RoCE PFC Statistics}
PFC statistics indicate a significant number of pause frames \autoref{fig:PFC_stats}. Combined with RTT peaks, this substantiates periodic congestion in the RoCEv2 network. Considering that the network is fully provisioned and overall link utilization is low, the presence of congestion may seem puzzling at first. The workload structure explains it: only a limited subset of GPUs transmits at line rate at any given time, and RoCEv2 does not employ packet spraying, so it cannot fully exploit redundant paths. Occasional incasts and ECMP hotspots further contribute to the observed congestion.

% \TODO{shouldn't be a subfigure?}
% {\color{red}
% Mehryar: I was not sure if we had room to include a PFC plot, so to keep things brief I only included an overview "PFC Statistics" table which is currently labeled as Figure 18. However, if deemed beneficial, please feel free to include the file SCALA\_ROCE\_PFC\_Plot.png, which you will find in the "figures" subdirectory (though not included in the paper). The plot shows further detail beyond the "PFC Statistics" table, and shows at which point in the simulation the NICs were experiencing congestions (PFC XOFFs).
% }

\begin{figure}[htbp]
    \centering
    \begin{subfigure}[b]{\columnwidth}
        \centering
        \includegraphics[width=\textwidth]{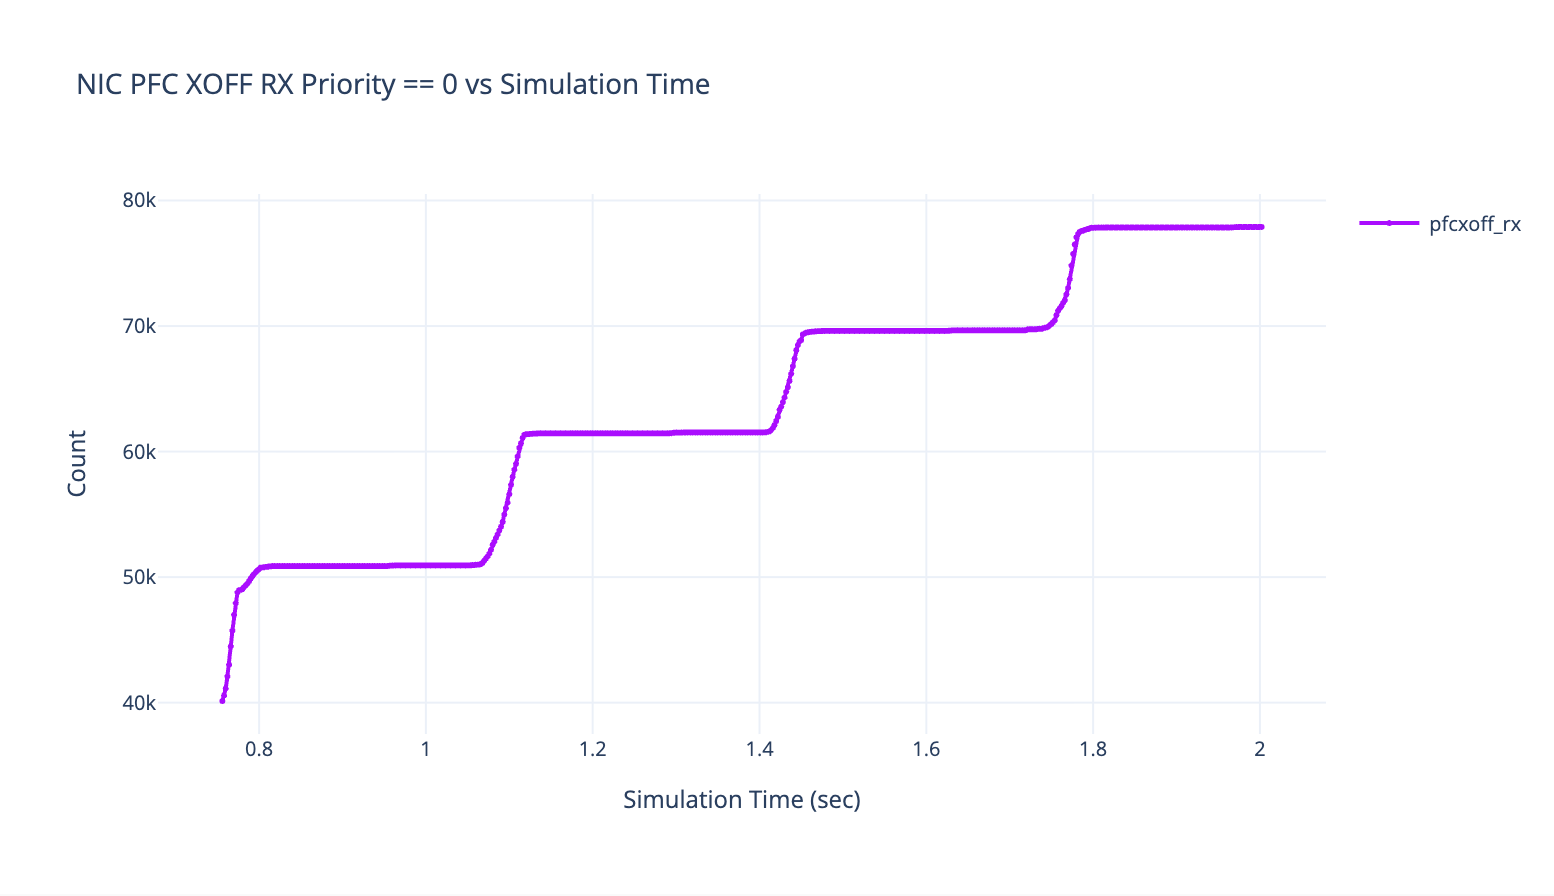}
        \caption{Congestion of ROCE PFC along with Timeline}
    \end{subfigure}
    \caption{PFC Statistics}
    \label{fig:PFC_stats}
\end{figure}

\begin{figure}[htbp]
    \centering
    \begin{subfigure}[b]{\columnwidth}
        \centering
        \includegraphics[width=\textwidth]{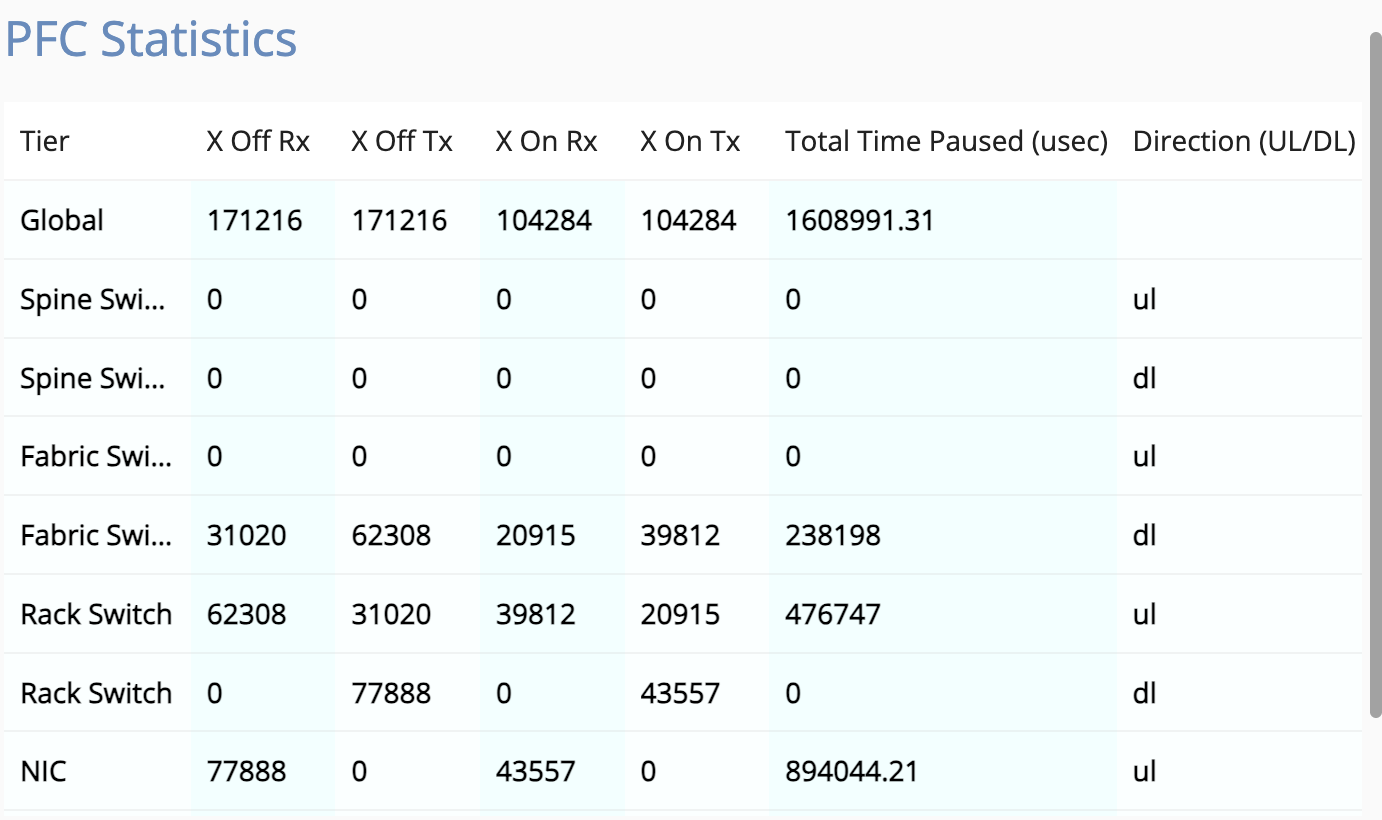}
        \caption{ROCEv2}
    \end{subfigure}
    \caption{PFC Statistics}
    \label{fig:PFC_stats}
\end{figure}

\subsubsection{eET NSCC Congestion Control}
For the eET transport, we observe a number of ECN M-marked packets, indicating occasional congestion \autoref{fig:congestio_control}. To manage this congestion, eET NSCC reduces the congestion window, as shown in the violin plot of eET congestion-window size. Despite these episodes of network congestion, NSCC appears effective at keeping RTT to a mean below 5 microseconds and a maximum below 26 microseconds throughout the run (see the eET RTT plot). Keeping network latency low is crucial for improving the performance of highly synchronized workloads such as LLMs on scale-out networks.

\begin{figure*}[htbp]
    \centering
    \begin{subfigure}[b]{0.45\textwidth}
        \centering
        \includegraphics[width=\textwidth]{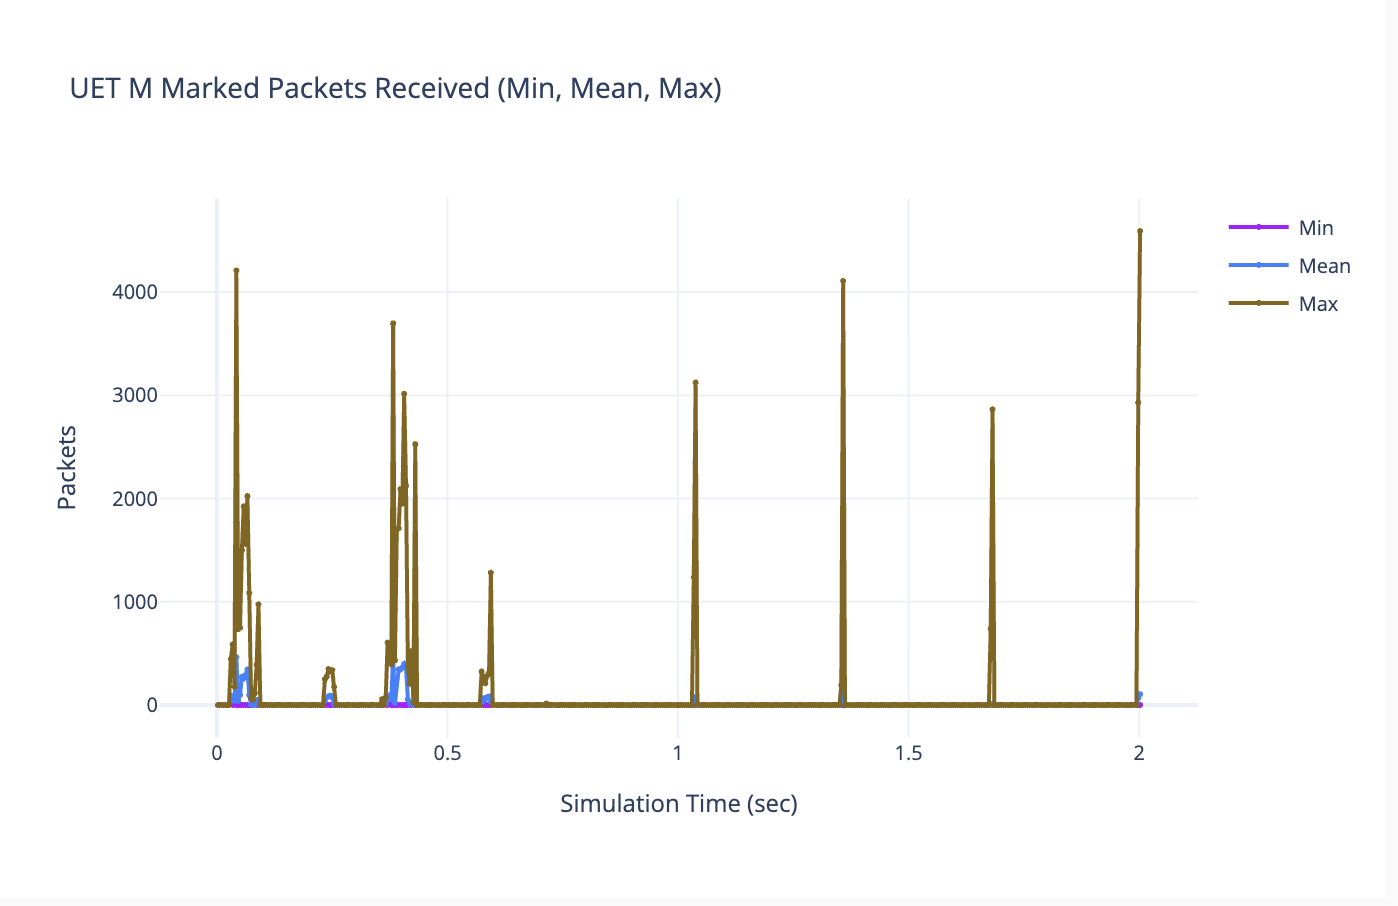}
        \caption{eET ECN M-Marked Packets}
    \end{subfigure}
    \hfill
    \begin{subfigure}[b]{0.45\textwidth}
        \centering
        \includegraphics[width=\textwidth]{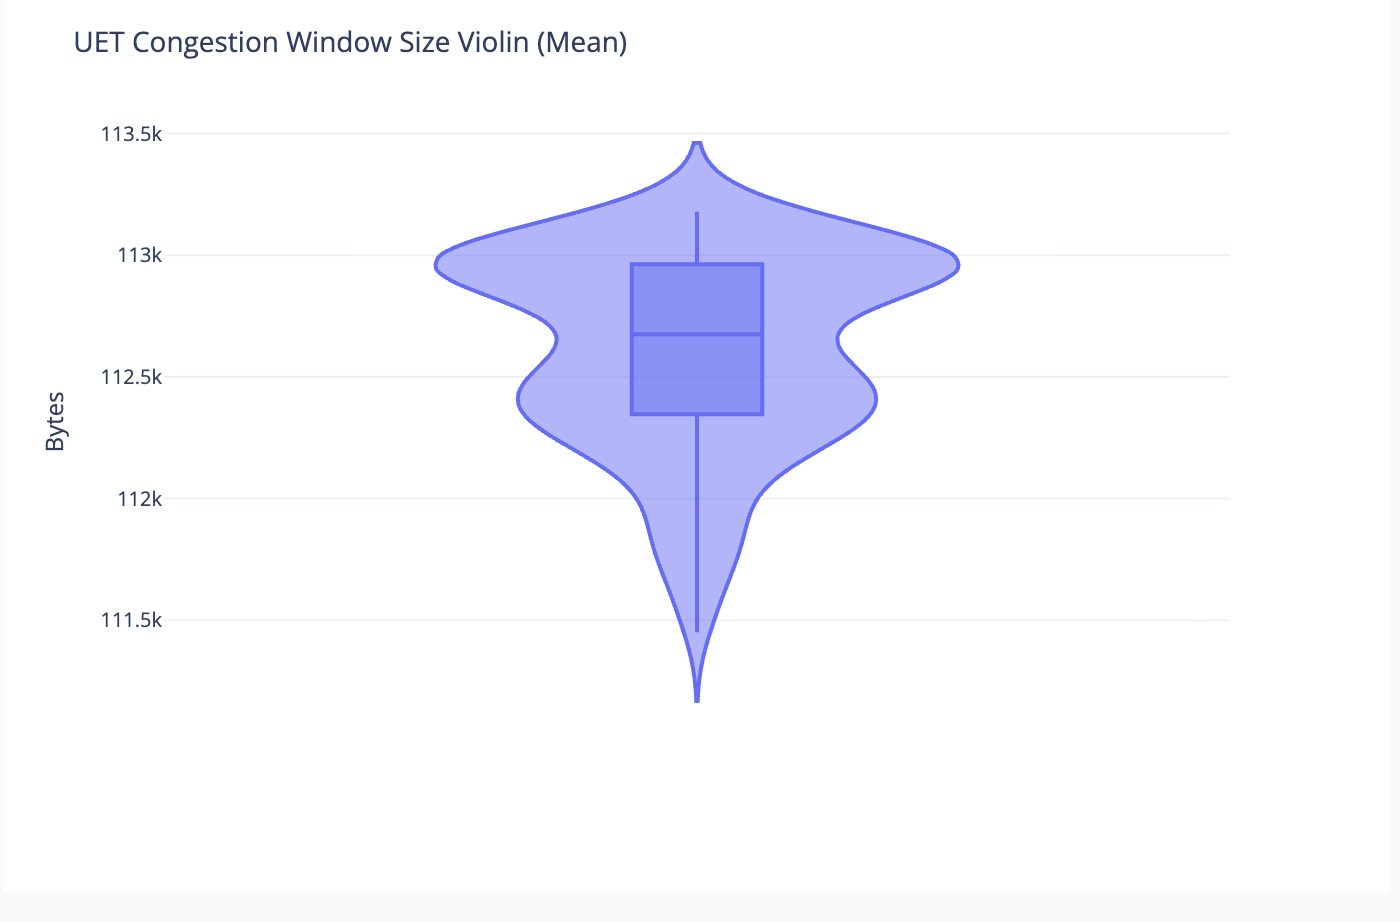}
        \caption{eET Congestion Window}
    \end{subfigure}
    \caption{eET NSCC Congestion Control}
    \label{fig:congestio_control}
\end{figure*}

\subsubsection{CDF for Send Bytes simulating NVIDIA A100}
The send-bytes cumulative distribution function (``Send Bytes CDF'') plots show the progression of the simulation within the allotted two-second time limit (shown in \autoref{fig:send_byte-A100}). Because the simulation time was capped at two seconds, the run ended before all Chakra traces finished executing. For RoCEv2, the CDF indicates that 7.84\% of the workload’s total bytes were sent; for eET, 7.96\% were sent. Thus, despite eET’s performance enhancing features relative to RoCEv, such as 128\hyp{}way sprays and lower tail latency achieved via eET NSCC versus RoCEv2 PFC, these did not translate into a net performance improvement for eET in this particular simulation. This may seem counterintuitive at first, but further analysis shows that the bottleneck was not network communication; rather, computation on the GPUs limited overall workload performance.

\begin{figure*}[htbp]
    \centering
    \begin{subfigure}[b]{0.45\textwidth}
        \centering
        \includegraphics[width=\textwidth]{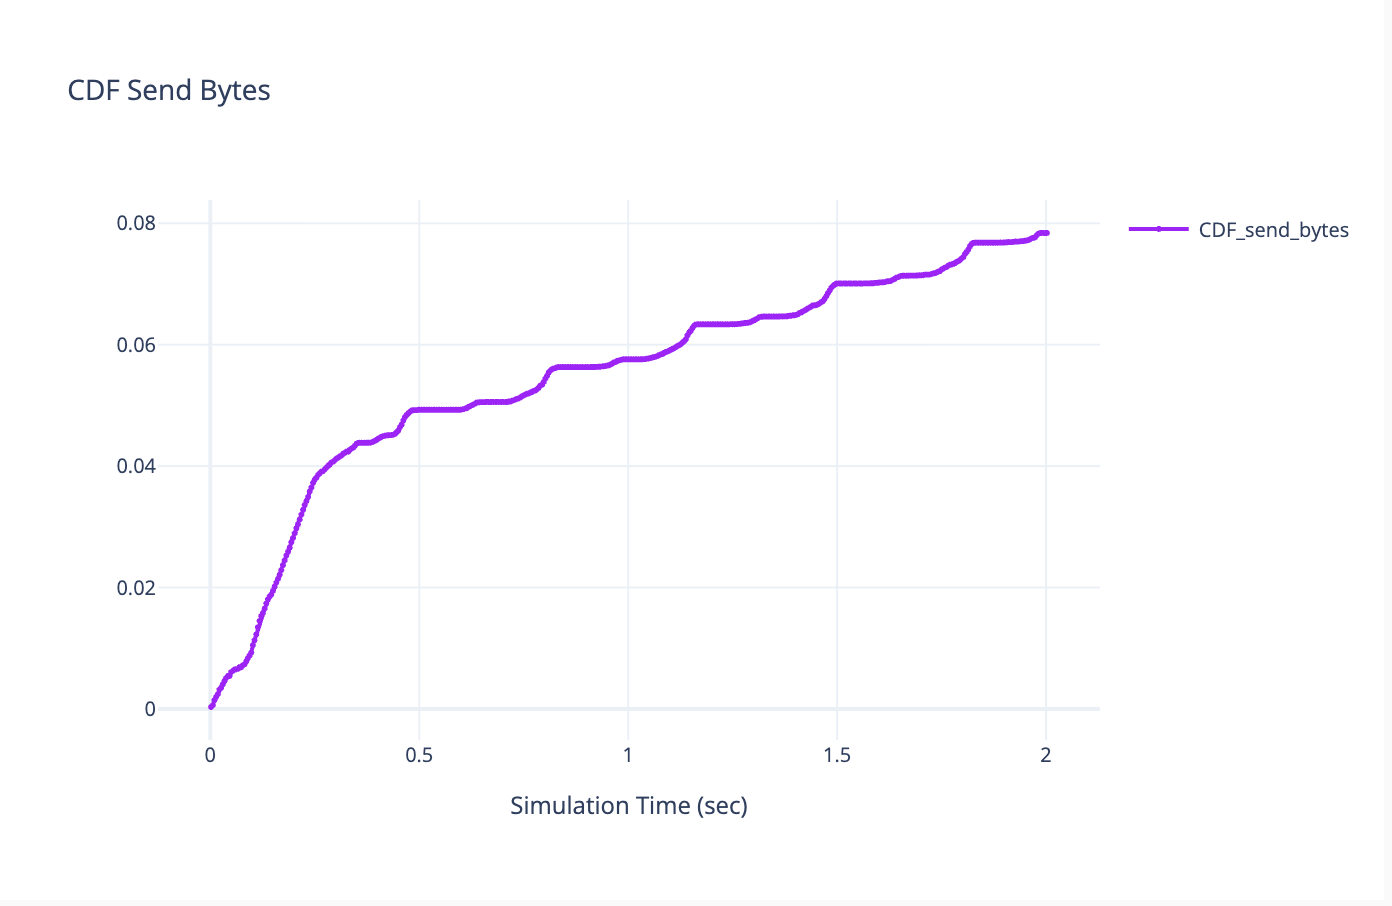}
        \caption{ROCEv2}
    \end{subfigure}
    \hfill
    \begin{subfigure}[b]{0.45\textwidth}
        \centering
        \includegraphics[width=\textwidth]{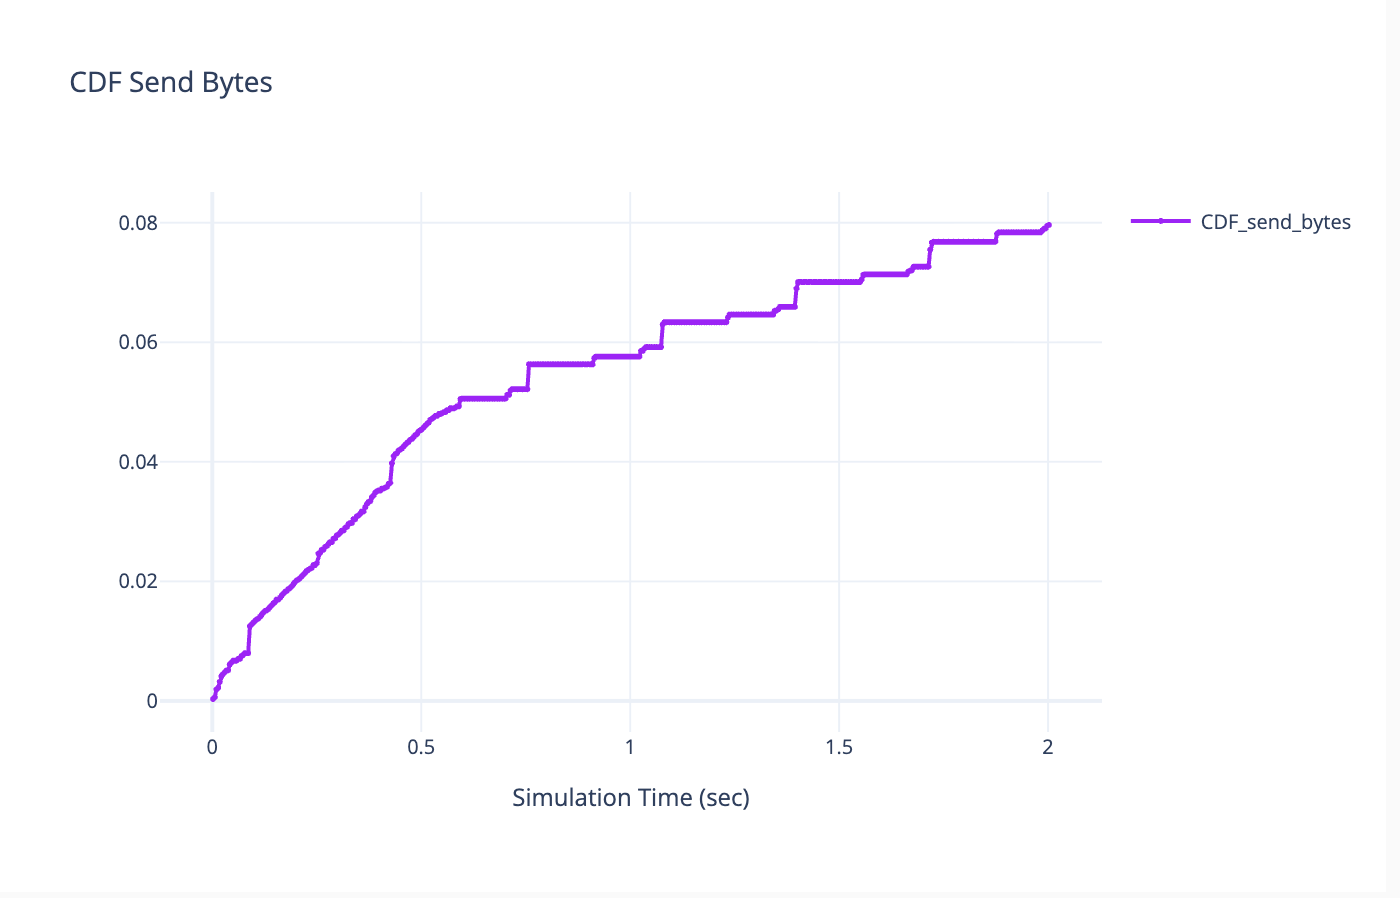}
        \caption{eET}
    \end{subfigure}
    \caption{Send Bytes Cumulative Distribution Function - A100}
    \label{fig:send_byte-A100}
\end{figure*}

\subsubsection{CDF for Send Bytes on Infinitely Fast GPU}
To validate that computation (not inter-GPU communication) is the limiting factor, we reran the simulation with all computation nodes’ \texttt{microDurations} attribute in the Chakra traces set to zero (shown in \autoref{fig:send_byte_infini}). This repeats the simulation under the assumption of an infinitely fast GPU that takes zero time to execute the computation nodes embedded in each Chakra trace. This assumption corresponds to an asymptotic case that we approach as we move from A100 to H100 to H200 and beyond. Under this assumption, we observe major differences between the performance of RoCEv2 and eET. In the RoCEv2 case, 17.4\% of the workload completed in two seconds. eET was significantly faster: 21.7\% of the workload completed in the same two seconds. These results validate that computation is indeed the performance-limiting factor.

Examining the CDF plots for the A100, two regions are apparent. In the initial region, before the simulation time reaches 300\,ms for RoCEv2 and 500\,ms for eET, the workload completes at a faster rate. Thereafter, execution slows markedly as the simulation enters a regime in which computation plays a larger role, reducing the likelihood that the network is the bottleneck. This slowdown is not observed when simulating an infinitely fast GPU: the workload’s send-bytes metric progresses with a nearly constant, single slope.

\begin{figure*}[htbp]
    \centering
    \begin{subfigure}[b]{0.45\textwidth}
        \centering
        \includegraphics[width=\textwidth]{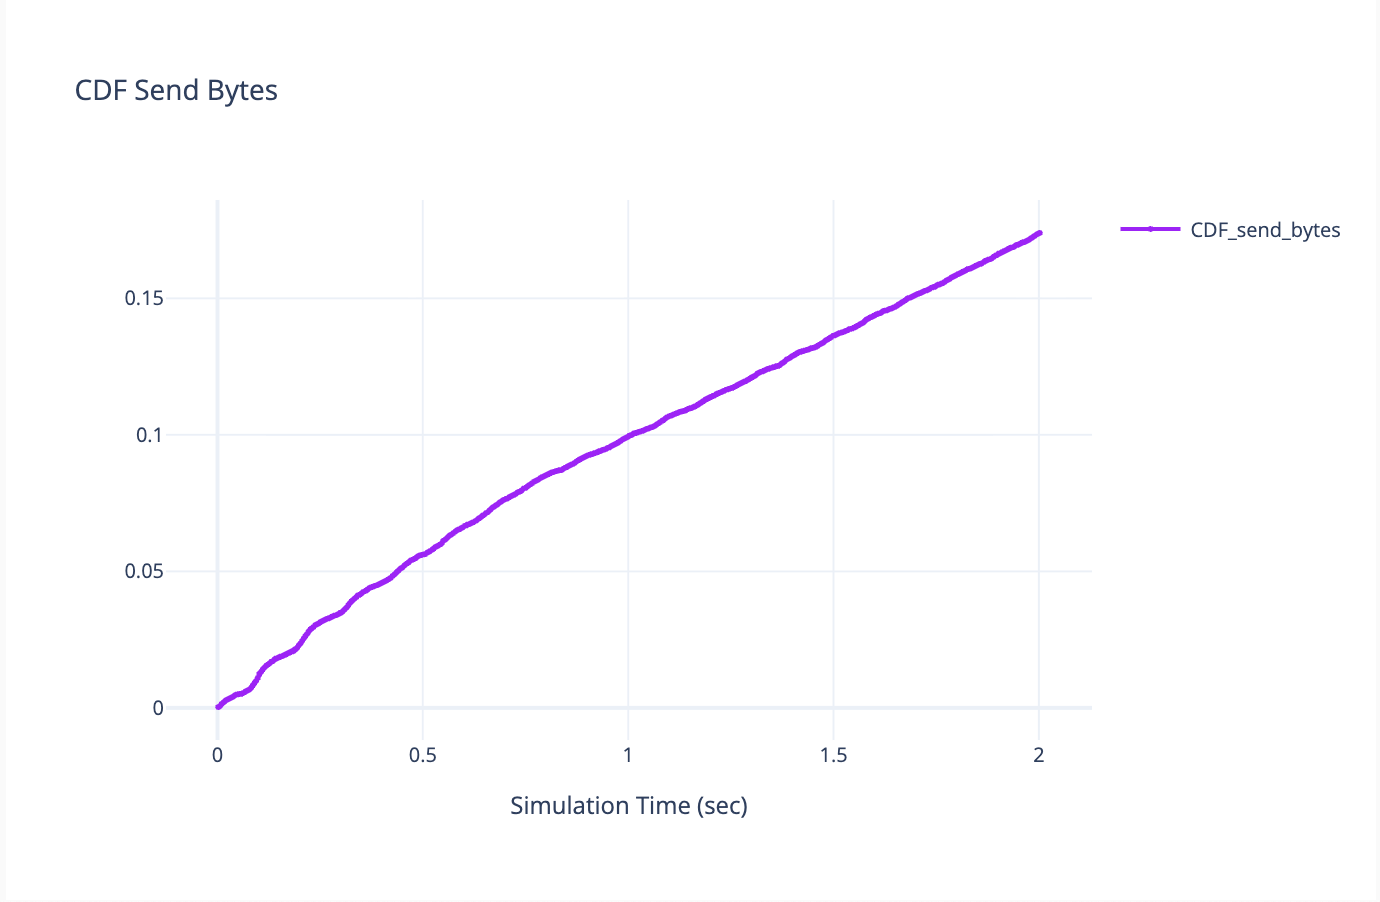}
        \caption{ROCEv2}
    \end{subfigure}
    \hfill
    \begin{subfigure}[b]{0.45\textwidth}
        \centering
        \includegraphics[width=\textwidth]{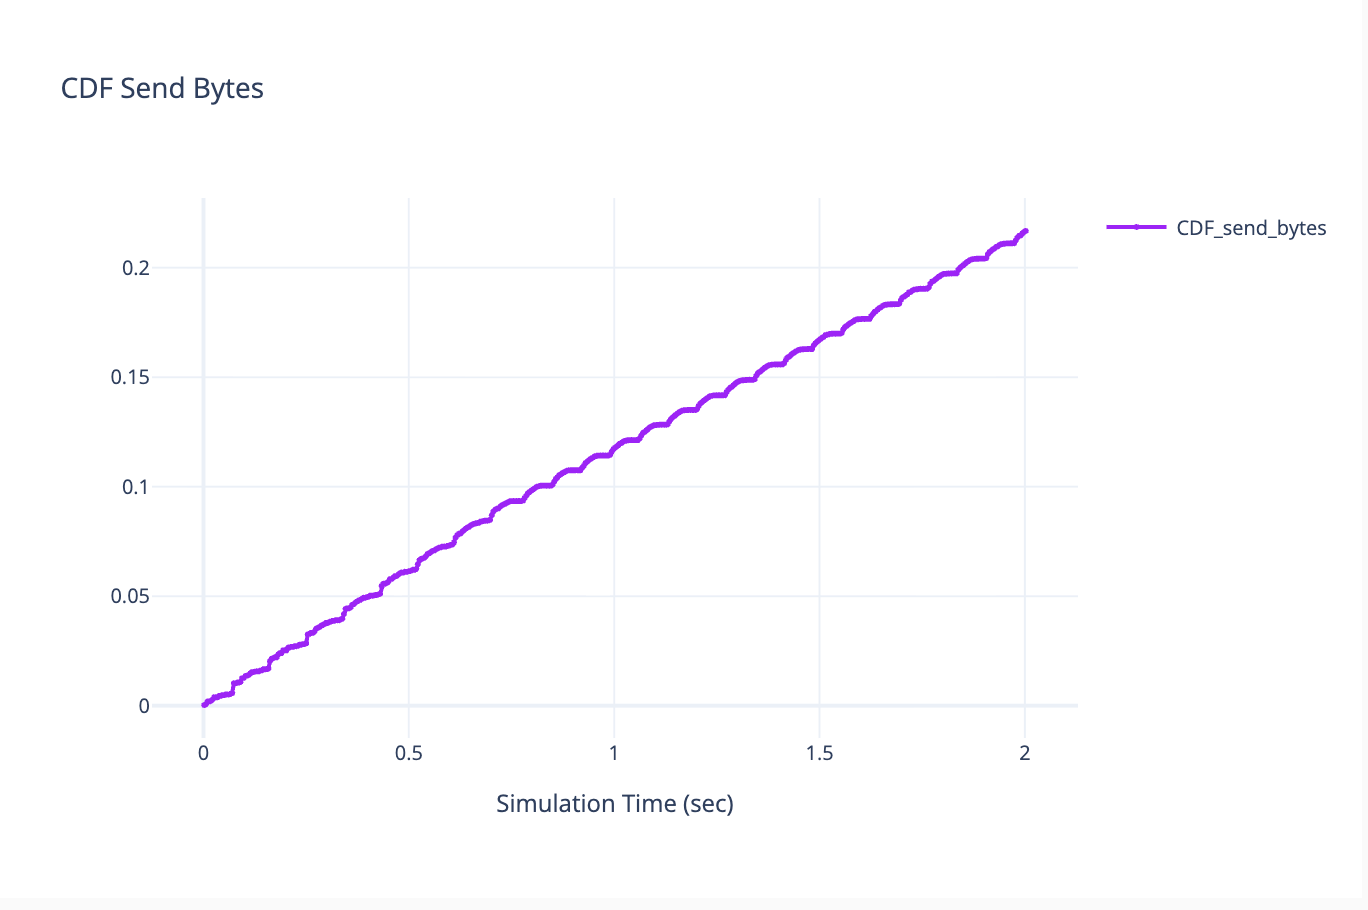}
        \caption{eET}
    \end{subfigure}
    \caption{Send Bytes Cumulative Distribution Function - Infinitely Fast GPU}
    \label{fig:send_byte_infini}
\end{figure*}

\subsubsection{Key Takeaways}
\begin{itemize}
  \setlength{\itemsep}{2pt}   % space between items
  \setlength{\parsep}{0pt}    % extra paragraph space within items
  \setlength{\parskip}{0pt}   % paragraph skip (often already 0)
  \setlength{\topsep}{0pt}    % space above/below the list
  \item LLM workloads are highly synchronized; execution speed depends not only on the transport protocol but also on the workload’s fine-grained structure and the interplay between communication and computation tasks.
  \item Given the nature of LLM workloads, RDMA transports that achieve lower latency or exploit redundant network paths generally perform better, so long as computation is not the bottleneck. 
  \item Chakra provides an effective way to capture dependencies within and across GPUs, enabling fine-grained simulation of LLM workloads over RDMA.
  \item Large-scale (100k+ GPU) network simulators enabled by Chakra, such as the Scala Computing platform, allow investigation of LLM workloads at scale and help identify performance bottlenecks in workload design and transport, yielding substantial savings in AI training and inference.
\end{itemize}
