# Supplementary material for: MLCommons Chakra: Advancing Performance Benchmarking and Co-design using Standardized Execution Traces
Source: arXiv:2605.11333 source file (2026-05-19)
Supplement: Supplementary file 2 [file appendix_discussion.tex]

\newpage
\section{Appendix B: Ongoing Chakra Extensions}
\label{sec:discussion}
\vspace{-1mm}

\subsection{Handling Large-Scale Traces}
\vspace{-1mm}
The Chakra framework prioritizes completeness and fidelity in trace representation, which is essential for accurate performance modeling and replay. For very large workloads, such as billion-parameter language models or training runs with millions of operations, this design choice results in execution traces that can span multiple gigabytes. While these trace sizes reflect the true complexity of modern ML workloads, they also present practical challenges for storage, exchange, and initial loading. This approach represents an intentional trade-off: preserving full operational detail enables high-fidelity simulation and faithful bottleneck analysis, which would be compromised by lossy compression or aggressive summarization. To improve usability at scale without sacrificing fidelity, future enhancements could include optional lossless compression for storage and transfer, alongside hierarchical indexing to enable partial loading and selective replay. Such optimizations would enhance the scalability of the framework while maintaining its core accuracy guarantees for large-scale analysis.

\subsection{Infrastructure Abstraction}
\vspace{-1mm}
Building on the system optimization capabilities discussed so far, trace-driven co-design requires complementary standardization of infrastructure descriptions.
While Chakra provides a standardized representation for workload execution traces, current infrastructure configurations rely on tool-specific formats that hinder portability and cross-platform comparison.
Just as Chakra enables workload exchange without exposing proprietary model details, a standardized infrastructure abstraction would allow hardware configurations to be shared and evaluated systematically across research teams and organizations.

Graph-based infrastructure representations that model compute nodes, memory hierarchies, and interconnect topologies in a structured, portable format offer a promising direction. Such an abstraction would naturally complement Chakra's execution graph model, enabling infrastructure-aware performance projection and topology-sensitive scheduling studies. When paired with Chakra ETs, standardized infrastructure descriptions could support cross-platform trace reuse, comparative analysis of interconnect designs, and feasibility assessments for parallelization strategies under realistic resource constraints.

Building this capability requires community engagement to establish schema requirements, develop converters for existing simulator formats, and validate portability across diverse toolchains. This represents a natural evolution of the Chakra ecosystem that would further strengthen its role in enabling reproducible, infrastructure-aware co-design for next-generation AI systems.
InfraGraph is an emerging effort within the MLCommons Chakra Working Group in this direction that complements Chakra by providing graph-based infrastructure modeling for the trace ecosystem.

\subsection{Chakra for MLPerf Storage}
\vspace{-1mm}
The MLPerf Storage benchmark ~\cite{mlperf-storage} suite measures how fast storage systems can supply training data when a model is being trained. Current implementation of the benchmark replaces all compute and communication with a fixed delay and only replays storage operations. This limits ability to replay compute/communications operations in a fine-grain manner with storage as well as adapt traces to different systems in a portable manner. We are currently working with MLPerf Storage working group to add storage operations to Chakra ETs and use Chakra replay for MLPerf Storage benchmarking.
